# Supplementary material for: An Energy-based Model for Word-level AutoCompletion in Computer-aided Translation
Source: arXiv:2407.20083 source file (2024-07-29)
Supplement: Supplementary file 1 [file appendix.tex]

% \section{Appendix}
% \subsection{Simulated Training Data}
% \label{appendix:simulated_training_data}
% Specifically, given a raw parallel sentence pair $(\boldsymbol{x},\boldsymbol{y})$, where $\boldsymbol{x} = (x_1, ..., x_m)$ is the source sentence, $\boldsymbol{y} = (y_1, ..., y_n)$ is the reference target sentence, we would like to construct a target word $w$ and its corresponding target context $\boldsymbol{c}=(\boldsymbol{c}_{l}, \boldsymbol{c}_{r})$ and human-typed characters $\boldsymbol{s}$, where the translation pieces $\boldsymbol{c}_{l}$ and $\boldsymbol{c}_{r}$ are on the left and right side of the target word $w$.

% According to \citet{li2021gwlan}, we first randomly sample a target word $w = \boldsymbol{y}_{t}$, and then we sample four types of context types:
% \begin{itemize}
%     \item Zero-context: both $\boldsymbol{c}_{l}$ and $\boldsymbol{c}_{r}$ are empty;
    
%     \item Prefix: randomly sample a translation piece $\boldsymbol{c}_{l}=\boldsymbol{y}_{i:j}$ from $\boldsymbol{y}$, where $i < j < t$. The $\boldsymbol{c}_{r}$ is empty.
    
%     \item Suffix: randomly sample a translation piece $\boldsymbol{c}_{r}=\boldsymbol{y}_{i:j}$ from $\boldsymbol{y}$, where $ t < i < j$. The $\boldsymbol{c}_{l}$ is empty. 
%     \item Bi-context: sample $\boldsymbol{c}_{l}$ as in prefix, and sample $\boldsymbol{c}_{r}$ as in suffix.
% \end{itemize}

% Last but not least, we need to generate human-typed characters $\boldsymbol{s}$ for the target word $w$, we adopt a heuristic method - we randomly sample a position $i$ in the target word $w$, where $0< i < |w|$, and simulate human-typed characters $\boldsymbol{s} = w_{1:i}$. For languages like Chinese, the human input is the phonetic symbols of the word, we use pypinyin\footnote{\url{https://github.com/mozillazg/python-pinyin}} to implement this conversion. So far, we get the tuple $(\boldsymbol{x}, \boldsymbol{c}, \boldsymbol{s}, w)$, which can be viewed as a simulated training example for WLAC task.

% \subsection{Detailed Results}
% \input{tables/detailed_results}
